# Supplementary material for: Zero-shot sim-to-real transfer of tactile control policies for aggressive swing-up manipulation
Source: arXiv:2101.02680 ancillary file (2021-05-06)
Supplement: Supplementary file 1 [file ExperimentalReport.pdf]

# Zero-shot sim-to-real transfer of tactile control policies for aggressive swing-up manipulation

## Experimental Report

Thomas Bi, Carmelo Sferrazza and Raffaello D’Andrea

| Pole  | $r$ [mm] | $l$ [mm] | $m$ [g] | MAE [deg]  | Failures     |
|-------|----------|----------|---------|------------|--------------|
| 1     | 2.5      | 200      | 28      | 5.6        | 29% (4/14)   |
| 2     | 2.5      | 350      | 38      | 3.5        | 9% (1/11)    |
| 3     | 3.8      | 250      | 20      | 4.4        | 9% (1/11)    |
| 4     | 5.0      | 300      | 36      | 3.6        | 0% (0/10)    |
| Total |          |          |         | <b>4.3</b> | <b>11.7%</b> |

TABLE I

THIS TABLE LISTS THE FOUR POLES THAT ARE USED DURING THE EXPERIMENTAL EVALUATION, AND SPECIFIES THEIR PHYSICAL ATTRIBUTES. MOREOVER, THE MEAN ABSOLUTE ERROR (MAE) AND NUMBER OF FAILURES ARE LISTED.

**Abstract**—This report presents a quantitative analysis of employment of the control policy proposed in [1] on the physical system. In particular, the swing-up manipulation is performed ten times for each of four different poles. Results show that the control policy successfully generalizes to the poles of different dimensions and inertias. A mean absolute error of  $4.3^\circ$  is achieved.

### I. EXPERIMENTAL SETUP

The student tactile control policy is deployed on the physical system without any adaptation, i.e., the policy learned in simulation is directly transferred to the physical hardware. Four different poles are used throughout the experiments. The physical attributes of each pole are listed in Table I. For each pole, the student control policy is employed until ten successful swing-ups have been achieved. Failures, which are defined to be runs where the pole either falls or the cart is commanded to positions outside of the stroke, are also counted. During each run, the estimated orientation  $\hat{\phi}$ , as well as the control actions taken are recorded.

### II. RESULTS

Fig. 1 contains a plot for each of the poles. Each plot depicts the mean trajectory of the estimated orientation  $\hat{\phi}$  over time for the ten successful runs. Additionally, the sample standard deviation of the ten runs is shown in the shaded blue area. As can be seen, the student control policy yields repeatable behaviour and successfully swings the poles

The authors are members of the Institute for Dynamic Systems and Control, ETH Zurich, Switzerland. Email correspondence to Thomas Bi [bit@ethz.ch](mailto:bit@ethz.ch)

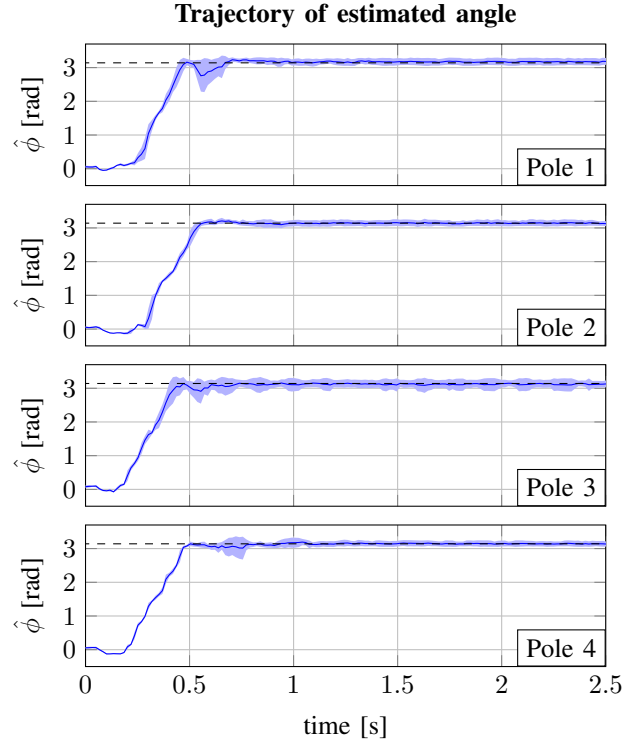

Fig. 1. This figure shows the trajectory of the estimated angle  $\hat{\phi}$  of the different poles when running the tactile control policy. For each pole, the control policy is run ten times. The resulting mean of the trajectory is shown by the solid blue line, while the shaded blue area depicts the standard deviation of the angle.

up to an angle of  $180^\circ$  with small offsets of the final angle. The time to reach the upright position is roughly equal across the four poles, with an average of  $\sim 0.5$  s. Additionally, there is only minimal overshoot.

Next, Fig. 2 shows the commanded cart acceleration and clamping distance for each pole averaged over the ten successful runs. As can be seen, the clamping range for poles of different radii naturally differ. It is important to note that these differences in the clamping distance arise purely from the feedback of the tactile sensor (i.e. the estimated orientation and total normal force), and that the radius is not known to the policy. Further, even for the two poles that share an identical radius (poles 1 and 2), there are noticeable differences in the commanded clamping distance (at around

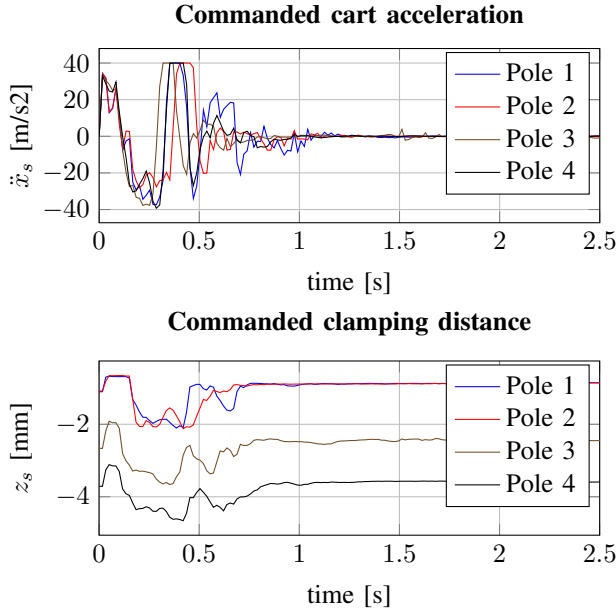

Fig. 2. This figure shows the control actions taken by the robotic system for the different poles, i.e. the commanded acceleration and the commanded clamping distance of the tactile gripper. For each pole, the mean values over the ten logged runs are shown. As can be seen from the commanded clamping distance, the difference in the radii of the poles lead to large offsets in the commanded clamping distances. Moreover, even for poles of the same radii (poles 1 and 2), the clamping distance trajectories differ due to the difference in inertia.

0.5 s). This can be attributed to the fact that due to the differences in the moment of inertia, different impulses are necessary to generate a sufficient angular momentum of the pole.

Finally, Table I also summarizes the results and states the mean absolute error (MAE) of the final estimated angle  $\hat{\phi}$  with a goal of  $180^\circ$ . Averaged over all the successful runs of the four poles, an error of  $4.3^\circ$  is observed. Moreover, the errors are consistent across the different poles. At this point, it is important to note that the estimated orientation is based on a  $20 \times 20$ -dimensional sensed force distribution, and may thus be noisy and does not necessarily provide ground truth.

It can also be seen that pole 1 experiences a higher failure rate when compared to the other three poles. From observing the trajectories for pole 1, it was seen that a restitution effect takes place once the pole reaches the upright position. In other words, the pole springs back slightly once it reaches the upright position. The control policy then attempts to correct for this behaviour by accelerating the cart (see seconds 0.5 – 0.75 in Fig. 2). This is also visible in the first plot of Fig. 1, where there is a small downward spike of the estimated angle at  $\sim 0.6$  s. The high accelerations then occasionally cause a motion that is too jerky, causing the gripper to lose contact with the pole, ultimately leading to failure. Further, the fact that this restitution effect is more pronounced for pole 1, can be attributed to the fact that the pole is relatively short, and thus its center of mass is closer to the point of contact on the tactile gripper. As a result, higher forces are necessary to generate the torques necessary to achieve the desired motion.

## REFERENCES

- [1] T. Bi, C. Sferrazza, and R. D’Andrea, “Zero-shot sim-to-real transfer of tactile control policies for aggressive swing-up manipulation,” *arXiv:2101.02680*, 2021.
